# Supplementary material for: Modelling crypto markets by multi-agent reinforcement learning
Source: arXiv:2402.10803 source file (2024-02-16)
Supplement: Supplementary file 1 [file 070_supplementary.tex]

\section{Supplementary material}
\label{SectionVII}
